# Supplementary material for: People construct simplified mental representations to plan
Source: arXiv:2105.06948 ancillary file (2022-11-26)
Supplement: Supplementary file 1 [file supplementary_information.pdf]

# *People construct simplified mental representations to plan*

## Supplementary Information

Mark K. Ho[1,2], David Abel[3], Carlos G. Correa[4], Michael L. Littman[3], Jonathan D. Cohen[1,4], and Thomas L. Griffiths[1,2]

[1]Princeton University, Department of Psychology, Princeton, NJ, USA

[2]Princeton University, Department of Computer Science, Princeton, NJ, USA

[3]Brown University, Department of Computer Science, Providence, RI, USA

[4]Princeton University, Princeton Neuroscience Institute, Princeton, NJ, USA

# Supplementary Information Guide


**1 Supplementary Analyses** **3**

1.1 Supplementary Memory Experiment Analyses . . . . . . . . . . . . . . . . . . . . 3

1.1.1 Up-front planning experiment: Interactions between execution and predictors . . . . . . . . . . . . . . . . . . . . . . . . . . . . . . . . . 3

1.1.2 Critical mazes experiment: Critical/irrelevant obstacle comparison . . . . . 4

1.2 Supplementary Control Experiment Analyses . . . . . . . . . . . . . . . . . . . . 4

1.2.1 Perceptual Control Analyses . . . . . . . . . . . . . . . . . . . . . . . 4

1.2.2 Execution Control Analyses . . . . . . . . . . . . . . . . . . . . . . . 5

1.2.3 Combined Control Analysis on Experiments with Initial Mazes . . . . . . 7

1.3 Supplementary Construal Modification Analyses . . . . . . . . . . . . . . . . . . 7

1.3.1 Analysis of Computed Plan Biases . . . . . . . . . . . . . . . . . . . . . 7

1.3.2 Reanalysis of Planning Experiments . . . . . . . . . . . . . . . . . . . . 13

1.4 Supplementary Alternative Mechanisms Analyses . . . . . . . . . . . . . . . . . . 14

**2 Supplementary Discussion of Construal Optimization Algorithms** **15**

2.1 Construal as a search problem . . . . . . . . . . . . . . . . . . . . . . . . . . 15

2.2 An example: Incremental search for a satisficing construal . . . . . . . . . . . . 17

2.3 Results and discussion . . . . . . . . . . . . . . . . . . . . . . . . . . . . . . 18

**3 Supplementary Experimental Materials** **23**

# 1 Supplementary Analyses

## 1.1 Supplementary Memory Experiment Analyses

### 1.1.1 Up-front planning experiment: Interactions between execution and predictors

For the up-front planning experiment, we wanted to determine to what extent executing a plan influenced awareness judgment responses. To assess this, we analyzed whether awareness responses after execution differed from those before execution (but after planning) in relation to different predictors. Specifically, we fit a hierarchical "main-effects model" to both early termination and full trials with by-participant and by-maze random intercepts. Value-guided construal probability, nine alternatives, and whether a trial terminated early (sum-coded: early = $1$, full = $-1$) were set as main fixed effects. Note that we used optimal policy distance instead of navigation distance.

We then compared the main-effects model to models that each additionally included an interaction term between early termination and the following predictors: value-guided construal probability, trajectory-based search hit score, graph-based search hit score, and minimum optimal distance. If including an interaction term increases the fit, this indicates that execution affects how a predictor influences awareness judgments. Comparisons with value-guided construal probability and graph-based search hit score interactions showed no significant difference according to log-likelihood ratio tests ($\chi^2(1) = 1.01, p = 1.0$ and $\chi^2(1) = 1.67, p = 0.79$, respectively; p-values are Bonferroni corrected). This finding supports the hypothesis that processing reflecting value-guided construal occurs before plan execution.

The trajectory-based search hit score interaction resulted in a greater fit ($\chi^2(1) = 24.75, p = 2.6 \times 10^{-6}$; p-value is Bonferroni corrected), but note that since the corresponding main effect has a negative coefficient ($\beta = -0.033, \text{S.E.} = 0.006$) and the interaction has a positive coefficient ($\beta = 0.013, \text{S.E.} = 0.003$), this means early termination decreased the association with judgments. Finally, including the optimal navigation distance interaction led to a

greater fit ($\chi^2(1) = 12.15, p = 0.0020$). The corresponding main effect coefficient is negative ($\beta = -0.082, \text{S.E.} = 0.004$; p-value is Bonferroni corrected) and interaction is positive ($\beta = 0.009, \text{S.E.} = 0.003$), which similarly indicates that not executing a plan attenuates the association with distance to the optimal path. This suggests that judgments reflecting distance to an optimal path or an actual path taken (e.g., in the initial experiment) are at least partially attributable to execution itself, rather than planning.

#### 1.1.2 Critical mazes experiment: Critical/irrelevant obstacle comparison

We examined whether obstacles that were far from the optimal path, but relevant (i.e., "critical obstacles") would be associated with higher accuracy, confidence, and awareness than irrelevant obstacles. This is a unique qualitative prediction of value-guided construal relative to the alternatives we consider (in particular, the heuristic search algorithms). We ran hierarchical linear/logistic models with by-participant random effects and whether an obstacle was critical or irrelevant as a fixed effect (relevant, but non-critical obstacles were not included in this analysis) and compared it to a model without the critical/irrelevant fixed effect. For all three measures, including the critical/irrelevant fixed effect fit the responses significantly better, using log-likelihood ratio tests (correct recall: $\chi^2(1) = 37.02, p = 1.2 \times 10^{-9}$; confidence: $\chi^2(1) = 53.57, p = 2.5 \times 10^{-13}$; awareness: $\chi^2(1) = 45.39, p = 1.6 \times 10^{-11}$).

### 1.2 Supplementary Control Experiment Analyses

#### 1.2.1 Perceptual Control Analyses

We wanted to determine whether value-guided construal predicts awareness judgments in the original planning experiments to which the control experiments were yoked better than the perceptual controls themselves. To assess this, we fit hierarchical linear models that included value-guided construal predictions, experiment (sum coded: original planning experiment = 1, perceptual control experiment = -1) and their interaction as fixed effects. The model also included

by-participant and by-maze random intercepts, unless it was singular, in which case only by-participant intercepts were included.

Recall that the perceptual control experiment using the initial set of mazes had viewing times yoked to the up-front planning experiment initial response times. For the hierarchical linear models fit to those responses, the value-guided construal / experiment interaction term was significant according to a log-likelihood ratio test ($\chi^2(1) = 950.19, p = 1.2 \times 10^{-208}$). Additionally, the coefficient associated with the main effect of value-guided construal was positive ($\beta = 0.057, \text{S.E.} = 0.002$) as was the interaction term ($\beta = 0.052, \text{S.E.} = 0.002$). This indicates that value-guided construal is more strongly associated with responses in the up-front planning experiment than in the yoked perceptual control.

The same type of analysis was done for accuracy, confidence, and awareness responses in the critical mazes experiment and the associated perceptual control experiment. Note that the awareness model only included by-participant random intercepts since otherwise it was singular. For all three measures, the value-guided construal / experiment interaction terms were significant according to log-likelihood ratio tests (accuracy: $\chi^2(1) = 51.50, p = 7.2 \times 10^{-13}$; confidence: $\chi^2(1) = 176.35, p = 3.0 \times 10^{-40}$; awareness: $\chi^2(1) = 675.93, p = 5.1 \times 10^{-149}$). Additionally, the coefficients associated with the main effect of value-guided construal were positive (accuracy: $\beta = 0.443, \text{S.E.} = 0.027$; confidence: $\beta = 0.064, \text{S.E.} = 0.003$; awareness: $\beta = 0.09, \text{S.E.} = 0.003$) as were the interaction terms (accuracy: $\beta = 0.195, \text{S.E.} = 0.027$ ; confidence: $\beta = 0.04, \text{S.E.} = 0.003$ ; awareness: $\beta = 0.086, \text{S.E.} = 0.003$ ). This indicates that value-guided construal is more strongly associated with responses in the planning experiment than in the yoked perceptual control.

### 1.2.2 Execution Control Analyses

Our first supplementary analysis of the execution controls was designed to test that obstacle distance to a participant's path taken (i.e., the navigation distance) was similar to in the original planning experiments. We calculated the correlation between mean navigation distances between

control and planning experiments, and found that they were highly correlated for both the initial set of mazes ($r(84) = 1.00, p = 1.5 \times 10^{-139}$) as well as the critical mazes ($r(20) = 1.00, p = 2.9 \times 10^{-24}$).

Additionally, as with the perceptual controls, we wanted to determine whether value-guided construal predicts awareness judgments in the original planning experiments to which the control experiments were yoked better than the execution controls themselves. To assess this, we fit hierarchical linear models that included value-guided construal predictions, experiment (sum coded: original planning experiment = 1, execution control experiment = -1) and their interaction as fixed effects. The model also included by-participant and by-maze random intercepts, unless it was singular, in which case only by-participant intercepts were included.

Recall that the execution control experiment using the initial set of mazes had breadcrumbs yoked to the initial planning experiment paths taken. For the hierarchical linear models fit to those responses, the value-guided construal / experiment interaction term was significant according to a log-likelihood ratio test ($\chi^2(1) = 120.89, p = 4.0 \times 10^{-28}$). Additionally, the coefficient associated with the main effect of value-guided construal was positive ($\beta = 0.114, \text{S.E.} = 0.002$) as was the interaction term ($\beta = 0.019, \text{S.E.} = 0.002$). This indicates that value-guided construal is more strongly associated with responses in the initial planning experiment than in the yoked execution control.

The same type of analysis was done for accuracy, confidence, and awareness responses in the critical mazes experiment and the associated execution control experiment. For all three measures, the value-guided construal / experiment interaction terms were significant according to log-likelihood ratio tests (accuracy: $\chi^2(1) = 60.41, p = 7.7 \times 10^{-15}$; confidence: $\chi^2(1) = 59.39, p = 1.3 \times 10^{-14}$; awareness: $\chi^2(1) = 97.10, p = 6.6 \times 10^{-23}$). Additionally, the coefficients associated with the main effect of value-guided construal were positive (accuracy: $\beta = 0.42, \text{S.E.} = 0.028$; confidence: $\beta = 0.078, \text{S.E.} = 0.003$; awareness: $\beta = 0.139, \text{S.E.} = 0.004$) as were the interaction terms (accuracy: $\beta = 0.215, \text{S.E.} = 0.028$ ; confidence: $\beta = 0.025, \text{S.E.} = 0.003$ ; awareness: $\beta = 0.037, \text{S.E.} = 0.004$ ). This indicates that value-guided construal is more strongly

associated with responses in the planning experiment than in the yoked execution control.

### 1.2.3 Combined Control Analysis on Experiments with Initial Mazes

In the main text, we reported analyses in which responses to the critical mazes were regressed onto mean responses to the control experiments. This was done in order to determine whether value-guided construal could explain planning responses above and beyond what could be accounted for by pure perception and execution. We performed the same analysis for awareness responses to the initial planning experiment and the up-front planning experiments.

Mean awareness responses for obstacles in the initial mazes on the control experiments were used as fixed effects in hierarchical linear models that included by-participant and by-maze random intercepts and were fit to responses from the initial experiment and up-front planning experiment. Each model was then compared to a version of the model that additionally included value-guided construal as a fixed effect using a log-likelihood ratio test. We found a significant change in fit for the initial experiment responses ($\chi^2(1) = 145.39, p = 1.8 \times 10^{-33}$) as well as the up-front planning experiment ($\chi^2(1) = 12.20, p = 0.00048$), and the coefficient on value-guided construal was positive (initial experiment: $\beta = 0.033, \text{S.E.} = 0.003$; up-front planning experiment: $\beta = 0.011, \text{S.E.} = 0.003$). This indicates that the results from the initial experiment and up-front planning experiment consistent with value-guided construal cannot be reduced to a combination of pure perception and execution.

## 1.3 Supplementary Construal Modification Analyses

### 1.3.1 Analysis of Computed Plan Biases

In addition to the *fixed parameter* and *fitted parameter* versions of the value-guided construal modification model reported in the main text, we fit models that incorporated the influence of biases at the level of computed plans, $\pi_c(a \mid s)$. Specifically, the models presented in the main text make the useful simplifying assumption that computed plans are noisy-optimal policies. How-

ever, people may have task-specific biases in how they plan at the action level, which can affect the value of different construals. For instance, in the mazes we use, although participants ultimately want to reach the goal state, they may have a slight bias to follow paths closer to the edge of the maze or may be especially averse to bumping into a wall. This would lead people to attend to obstacles that block otherwise optimal movements that are at the edge of the maze rather than ones closer to the center. Our goal in the current analyses is to show how such domain-specific factors can be incorporated into the more general framework of value-guided construal.

To account for potential biases in computed plans and how they might influence construal, we performed a grid search over two additional parameters along with the four $\varepsilon$-softmax parameters used for the original *fitted parameter* model (see Methods, Model Implementations, Value-Guided Construal; Figure 5 in the main text). The two new parameters included a cost based on weighting the Manhattan distance to the closest edge of the maze ($r_{\text{edge}} \in \{0., -0.01, -.1, -1.0\}$) and a cost for bumping into a wall or obstacle ($r_{\text{bump}} \in \{0, -0.1, -1.0\}$). The underlying reward function of the model of the task was then augmented with these values. We performed a grid search over 57,600 combinations of the 16 mazes and $r_{\text{edge}}, r_{\text{bump}}, \alpha_a^{-1}, \varepsilon_a, \alpha_c^{-1}$, and $\varepsilon_c$ values.

For each of the nine planning experiments/measures, we selected the set of parameters that produced the highest $R^2$ using a simple linear regression between the construal modification model outputs and mean by-obstacle responses. Supplementary Figures 1, 2, and 3 compare model predictions for the basic single value-guided construal model with $\alpha_c^{-1} = 10$; the fixed value-guided construal modification model that with optimal computed policies and $\alpha_c^{-1} = 10$; the fitted value-guided construal modification model with noise parameters $\alpha_a, \varepsilon_a, \alpha_c$, and $\varepsilon_c$; and the fitted value-guided construal modification model with additional computed plan bias parameters $r_{\text{edge}}$ and $r_{\text{bump}}$. Supplementary Tables 1 and 2 show the parameters for the two fitted value-guided construal modification models.

In general, we find that the fit between the model predictions and mean by-obstacle responses improves when the computed policy bias parameters are incorporated, where improvement varies by maze set and dependent measure. These analyses and results show how domain-specific biases

that shape computed plans can be incorporated into the value-guided construal framework in a principled manner. To be clear, we do not consider the two biases we examine here to exhaust the space of possible biases in computed plans. A key direction for future work will be identifying such biases in specific domains in a way that builds on the approach we apply here.

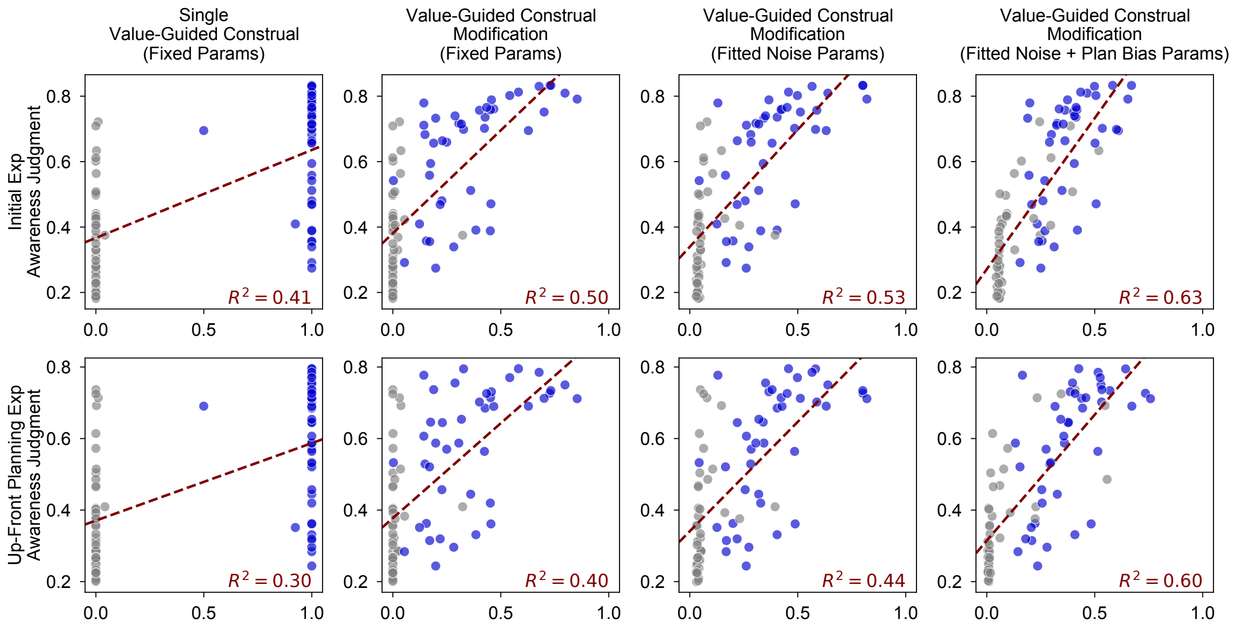


**Supplementary Figure 1:** Initial experiment and up-front planning experiment mean obstacle awareness responses compared to four increasingly elaborated versions of value-guided construal: the basic single value-guided construal model with $\alpha_c^{-1} = 10$; the fixed value-guided construal modification model with optimal computed policies and $\alpha_c^{-1} = 10$; the fitted value-guided construal modification model with noise parameters $\alpha_a, \varepsilon_a, \alpha_c$, and $\varepsilon_c$; and the fitted value-guided construal modification model with additional computed plan bias parameters $r_{\text{edge}}$ and $r_{\text{bump}}$. Grey and blue dots correspond to obstacles that the basic single value-guided construal model assigns probabilities below or above $0.1$, respectively.

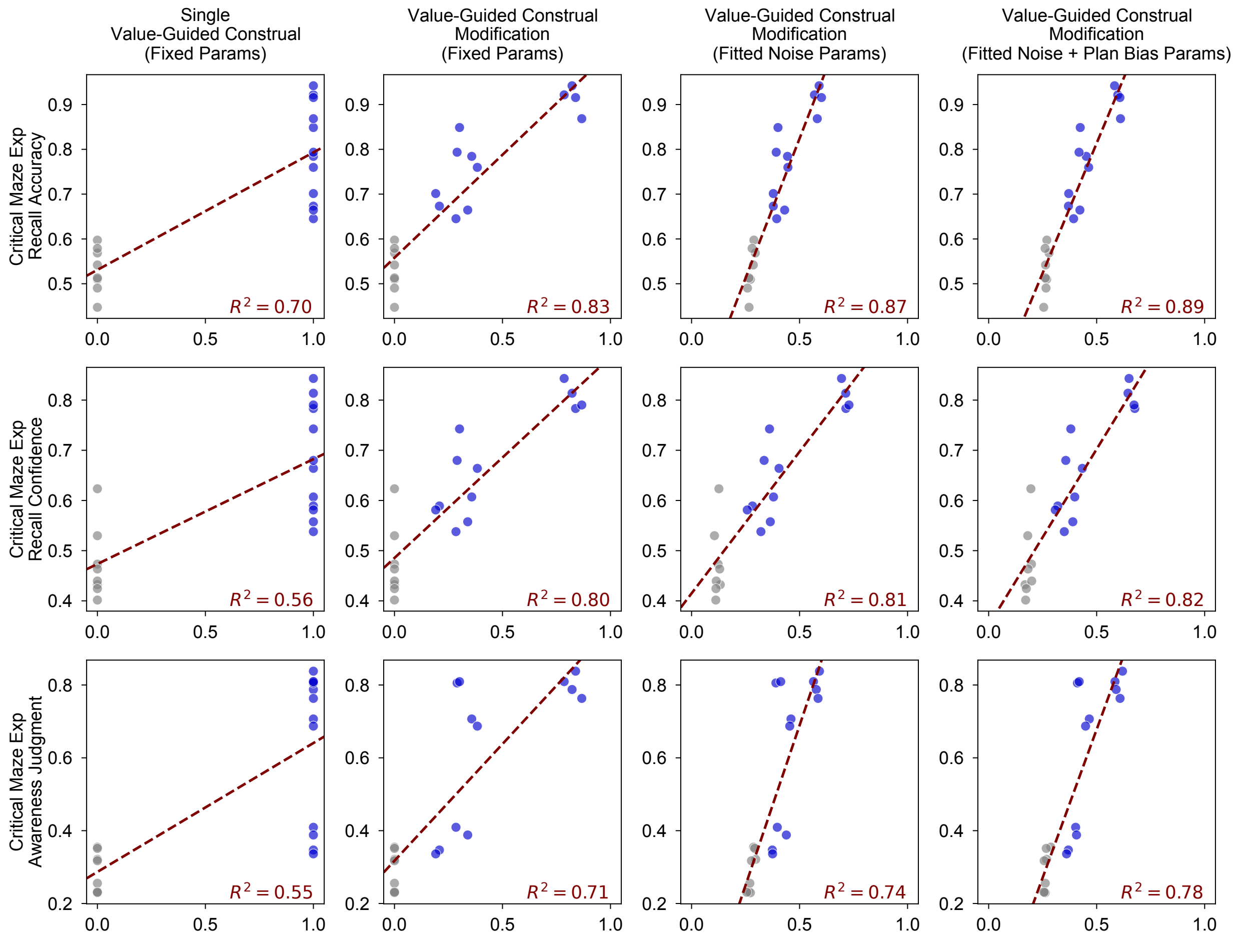


**Supplementary Figure 2:** Critical maze experiment mean obstacle accuracy, confidence, and awareness responses compared to four increasingly elaborated versions of value-guided construal: the basic single value-guided construal model with $\alpha_c^{-1} = 10$; the fixed value-guided construal modification model with optimal computed policies and $\alpha_c^{-1} = 10$; the fitted value-guided construal modification model with noise parameters $\alpha_a, \varepsilon_a, \alpha_c$, and $\varepsilon_c$; and the fitted value-guided construal modification model with additional computed plan bias parameters $r_{\text{edge}}$ and $r_{\text{bump}}$. Grey and blue dots correspond to obstacles that the basic single value-guided construal model assigns probabilities below or above $0.1$, respectively.

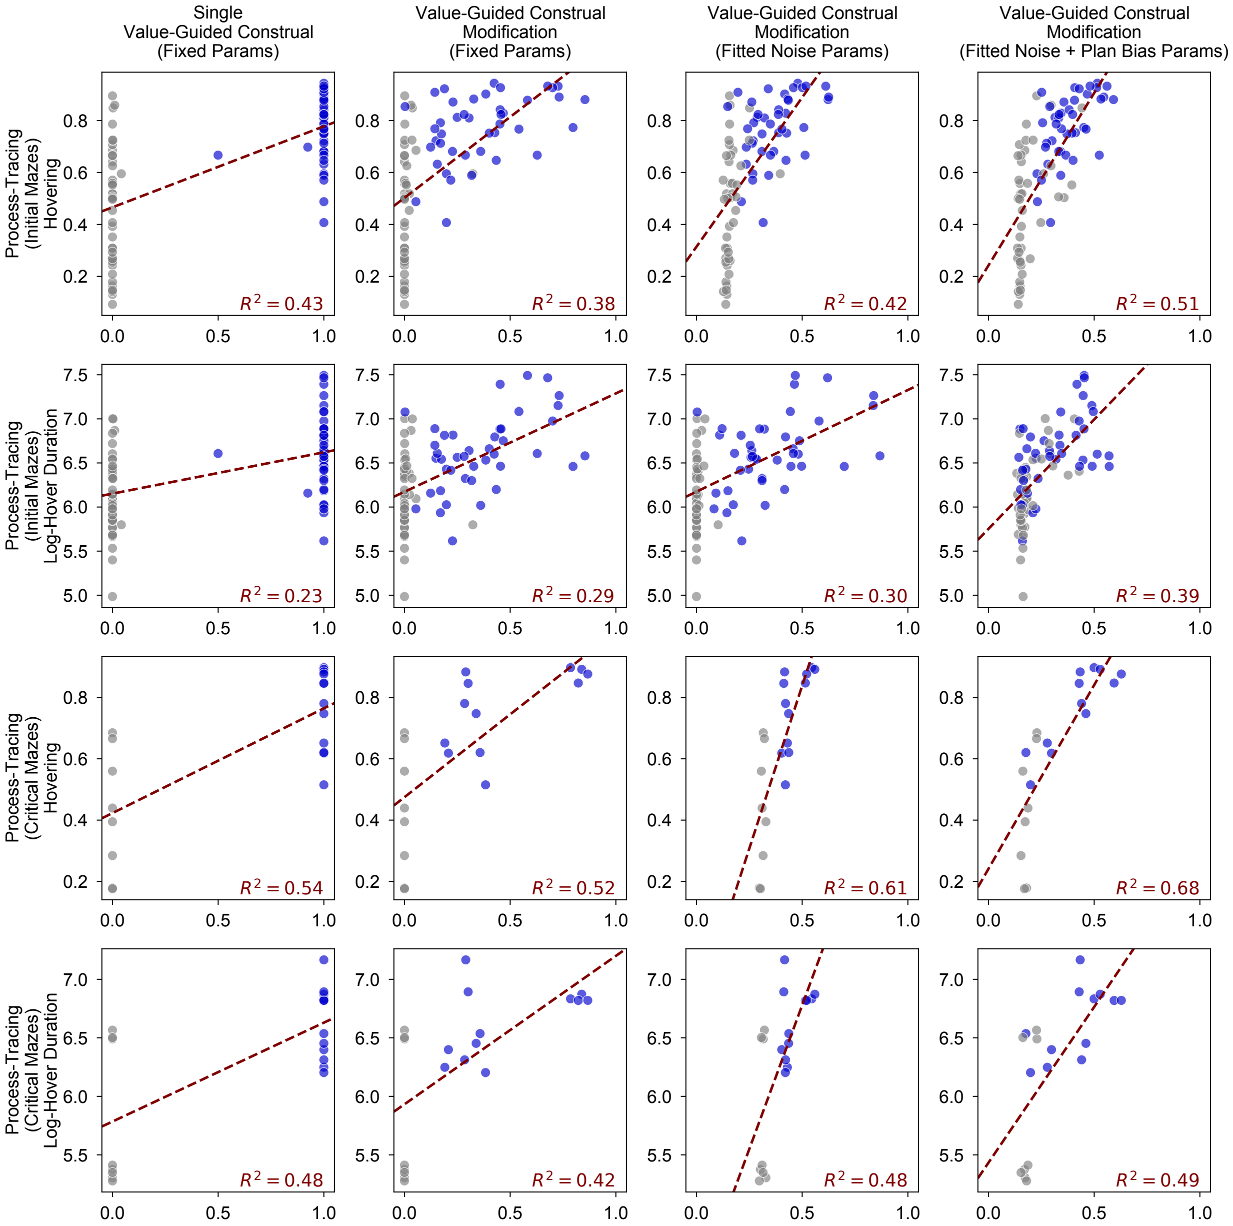


**Supplementary Figure 3:** Process-tracing experiment mean obstacle hovering and duration responses compared to four increasingly elaborated versions of value-guided construal: the basic single value-guided construal model with $\alpha_c^{-1} = 10$; the fixed value-guided construal modification model with optimal computed policies and $\alpha_c^{-1} = 10$; the fitted value-guided construal modification model with noise parameters $\alpha_a, \varepsilon_a, \alpha_c$, and $\varepsilon_c$; and the fitted value-guided construal modification model with additional computed plan bias parameters $r_{\text{edge}}$ and $r_{\text{bump}}$. Grey and blue dots correspond to obstacles that the basic single value-guided construal model assigns probabilities below or above $0.1$, respectively.

| | | $\alpha_a^{-1}$ | $\epsilon_a$ | $\alpha_c^{-1}$ | $\epsilon_c$ | $R^2$ |
|---|---|---|---|---|---|---|
| Initial Exp | Awareness | 1.00 | 0.20 | 5.00 | 0.05 | 0.53 |
| Up-Front Planning Exp | Awareness | 1.00 | 0.20 | 5.00 | 0.05 | 0.44 |
| Critical Maze Exp | Awareness | 3.00 | 0.10 | 1.00 | 0.05 | 0.74 |
| | Accuracy | 3.00 | 0.20 | 1.00 | 0.05 | 0.87 |
| | Confidence | 5.00 | 0.00 | 9.00 | 0.20 | 0.81 |
| Process-Tracing (Initial Mazes) | Duration | 1.00 | 0.00 | 9.00 | 0.00 | 0.30 |
| | Hovering | 7.00 | 0.20 | 7.00 | 0.30 | 0.42 |
| Process-Tracing (Critical Mazes) | Duration | 5.00 | 0.10 | 1.00 | 0.30 | 0.48 |
| | Hovering | 5.00 | 0.10 | 1.00 | 0.30 | 0.61 |

**Supplementary Table 1:** Fitted value-guided construal modification parameters.

| | | $\alpha_a^{-1}$ | $\epsilon_a$ | $\alpha_c^{-1}$ | $\epsilon_c$ | $r_{\text{edge}}$ | $r_{\text{bump}}$ | $R^2$ |
|---|---|---|---|---|---|---|---|---|
| Initial Exp | Awareness | 1.00 | 0.20 | 9.00 | 0.10 | -0.10 | -1.00 | 0.63 |
| Up-Front Planning Exp | Awareness | 1.00 | 0.20 | 5.00 | 0.00 | -0.10 | -1.00 | 0.60 |
| Critical Maze Exp | Awareness | 5.00 | 0.20 | 1.00 | 0.00 | 0.00 | -1.00 | 0.78 |
| | Accuracy | 3.00 | 0.10 | 1.00 | 0.00 | -0.01 | -1.00 | 0.89 |
| | Confidence | 3.00 | 0.10 | 5.00 | 0.30 | 0.00 | -1.00 | 0.82 |
| Process-Tracing (Initial Mazes) | Duration | 1.00 | 0.20 | 5.00 | 0.30 | -1.00 | 0.00 | 0.39 |
| | Hovering | 1.00 | 0.20 | 5.00 | 0.30 | -0.10 | -1.00 | 0.51 |
| Process-Tracing (Critical Mazes) | Duration | 1.00 | 0.00 | 9.00 | 0.30 | -1.00 | -0.10 | 0.49 |
| | Hovering | 1.00 | 0.00 | 9.00 | 0.30 | -1.00 | -0.10 | 0.68 |

**Supplementary Table 2:** Fitted value-guided construal modification parameters with computed plan biases.

### 1.3.2 Reanalysis of Planning Experiments

We ran a series of hierarchical generalized linear models using the fixed parameter value-guided construal modification model. These analyses were analogous to those with the single construal model. For all planning experiments and measures, we found that the fixed parameter value-guided construal modification model significantly predicted responses using likelihood ratio tests that compared models with and without value-guided construal as a fixed effect ( Initial Experiment Awareness: $\chi^2(1) = 2887.89, p < 1.0 \times 10^{-16}$; $\beta = 0.159$, S.E. $= 0.003$; Up-front Planning Experiment Awareness (F): $\chi^2(1) = 1059.32, p < 1.0 \times 10^{-16}$; $\beta = 0.149$, S.E. $= 0.004$; Up-front Planning Experiment Awareness (E): $\chi^2(1) = 877.32, p < 1.0 \times 10^{-16}$; $\beta = 0.128$, S.E.

$= 0.004$; Critical Mazes Experiment Accuracy: $\chi^2(1) = 341.59, p < 1.0 \times 10^{-16}$; $\beta = 0.728$, S.E. $= 0.045$; Critical Mazes Experiment Confidence: $\chi^2(1) = 633.71, p < 1.0 \times 10^{-16}$; $\beta = 0.1$, S.E. $= 0.004$; Critical Mazes Experiment Awareness: $\chi^2(1) = 1121.27, p < 1.0 \times 10^{-16}$; $\beta = 0.161$, S.E. $= 0.004$; Process-tracing on initial mazes hovering $\chi^2(1) = 1161.02, p < 1.0 \times 10^{-16}$; $\beta = 0.833$, S.E. $= 0.027$; Process-tracing on initial mazes hover duration [log milliseconds]: $\chi^2(1) = 287.87, p < 1.0 \times 10^{-16}$; $\beta = 0.211$, S.E. $= 0.012$; Process-tracing on critical mazes hovering: $\chi^2(1) = 1439.55, p < 1.0 \times 10^{-16}$; $\beta = 0.767$, S.E. $= 0.023$; Process-tracing on critical mazes hover duration [log milliseconds]: $\chi^2(1) = 466.32, p < 1.0 \times 10^{-16}$; $\beta = 0.247$, S.E. $= 0.011$).

In addition, we conducted the *combined control analyses* with the fixed parameter value-guided construal modification model. Data from the memory planning experiments were first fit to models that included mean by-obstacle responses to the perception and execution controls as fixed effects. We then compared the fit of these models with that of new models that included the fixed parameter value-guided construal modification predictions as a fixed effect. Consistent with the original analyses, for all measures, we found that the including the value-guided construal predictors increased fit and that the estimated coefficients were positive (Initial Experiment Awareness test and coefficient: $\chi^2(1) = 81.20, p = 2.0 \times 10^{-19}$, $\beta = 0.029, \text{S.E.} = 0.003$; Up-front Planning Experiment Awareness test and coefficient: $\chi^2(1) = 4.91, p = 0.027, \beta = 0.008, \text{S.E.} = 0.004$; Critical Maze Experiment Accuracy: $\chi^2(1) = 158.36, p = 2.6 \times 10^{-36}$, $\beta = 0.615, \text{S.E.} = 0.054$; Critical Maze Experiment Confidence: $\chi^2(1) = 15.12, p = 0.00010$, $\beta = 0.029, \text{S.E.} = 0.007$; Critical Maze Experiment Awareness: $\chi^2(1) = 5.12, p = 0.024$, $\beta = 0.017, \text{S.E.} = 0.007$).

## 1.4 Supplementary Alternative Mechanisms Analyses

In the main text, we reported hierarchical generalized linear regressions that tested the fixed parameter value-guided construal modification model alongside ten alternative predictors. We ran the same set of analyses except using the single construal version of the model and similarly

found that it remained a significant predictor even when accounting for the influence of alternatives (likelihood ratio tests between full global models and models without value-guided construal modification: Initial Exp, Awareness: $\chi^2(1) = 400.63, p < 1.0 \times 10^{-16}$; Up-front Exp, Awareness (F): $\chi^2(1) = 203.67, p < 1.0 \times 10^{-16}$; Up-front Exp, Awareness (E): $\chi^2(1) = 127.79, p < 1.0 \times 10^{-16}$; Critical Mazes Exp, Accuracy: $\chi^2(1) = 86.07, p < 1.0 \times 10^{-16}$; Critical Mazes Exp, Confidence: $\chi^2(1) = 173.12, p < 1.0 \times 10^{-16}$; Critical Mazes Exp, Awareness: $\chi^2(1) = 376.52, p < 1.0 \times 10^{-16}$; Process-Tracing Exp (Initial Mazes), Hovering: $\chi^2(1) = 289.13, p < 1.0 \times 10^{-16}$; Process-Tracing Exp (Initial Mazes), Duration: $\chi^2(1) = 89.71, p < 1.0 \times 10^{-16}$; Process-Tracing Exp (Critical Mazes), Hovering: $\chi^2(1) = 210.47, p < 1.0 \times 10^{-16}$; Process-Tracing Exp (Critical Mazes), Duration: $\chi^2(1) = 242.78, p < 1.0 \times 10^{-16}$). These results indicate that the broad qualitative effects of value-guided construal explain responses and provide additional support for our central hypothesis.

# 2 Supplementary Discussion of Construal Optimization Algorithms

Value-guided construal provides a normative [1–3] account of task representations during planning. As we have noted, our primary goal is to provide an account of optimality that serves as a benchmark and starting point for future algorithmic analyses of how people solve the problem of construal. In this section, we provide an initial illustration of how the value-guided construal framework can be extended to address algorithmic questions and also demonstrate the feasibility of tractably optimizing construals. We emphasize that specific claims about the algorithmic processes by which people optimize value-guided construals is beyond the present scope of this work.

## 2.1 Construal as a search problem

Recall that in our model of value-guided construal, the decision-maker starts with a set of effects $c \subseteq \{\phi_0, \phi_1, ..., \phi_n\}$ that can be combined to form a transition model, $P_c$, that is then used for

computing a plan, $\pi_c$. Then, the decision-maker wants to find a construal that optimizes the *value of representation*, $\text{VOR}(c) = U(\pi_c) - C(c)$. Thus, we can conceptualize construal optimization as a form of combinatorial search over subsets of effects (not to be confused with search over action sequences).

In the main Methods (under Model Implementations, Value-guided Construal), we present an *exhaustive* algorithm that generates and evaluates all possible construals. The main benefit of this approach is that it is guaranteed to return the globally optimal solution, and therefore provides a theoretical baseline with which to test our *normative* claim. However, exhaustive enumeration is an implausible account of the *algorithmic* process used to optimize construals. In particular, the exhaustive algorithm always generates the optimal plan for a construal that includes all candidate effects—that is, it always generates the plan for a fully specified task at some point. A more realistic algorithmic model would evaluate construals in a more targeted way—for instance, it would only solve the fully specified task if it were the only useful construal.

Can value-guided construals be computed non-exhaustively? We note that in general, whether certain classes of combinatorial optimization problems admit non-exhaustive algorithms depends on a number of factors, including the distribution of problems, the structure of the solution space, and the structure of the loss function. Similarly, non-exhaustive solutions can take on different forms—rather than optimizing, it may be sufficient to satisfice [4]; the algorithm may have a good way to initialize the optimization process; domain-specific heuristics may be available; etc. Finally, the same computational problem may have multiple algorithmic solutions that exhibit different trade-offs or are tailored for specific sub-domains. In the next section, we work through one family of algorithms that calculate construals non-exhaustively. Again, we emphasize that our aim here is not to propose an algorithmic account of how people optimize construals, but rather show that, in principle, construals can be computed relatively efficiently. This demonstration can serve as an impetus for future work that seeks to more specifically characterize how people solve the problem of finding good task representations.

## 2.2 An example: Incremental search for a satisficing construal

For a minimal demonstration of a non-exhaustive approach to identifying value-guided construals, we combined several ideas. First, we observed that because smaller construals are preferable, all other things equal, it makes sense to evaluate construals starting with the smallest one and then incrementally increase the number of effects considered. This induces a directed graph over construals: the empty construal has edges pointing to construals with one effect, each of which has arrows pointing to size 2 construals with another effect added, etc. Thus, starting from the empty construal, we can then perform search over the construal graph (not to be confused with search over action sequences). We then considered a set of search procedures that evaluate construals in more or less breadth-first versus depth-first order. Specifically, we designed a "bounded depth-first search by $n$" (B-DFS$(n)$) algorithm that performs depth-first search (DFS) up to a depth of $n$ and then afterwards performs breadth-first search (BFS). Note that BFS is then the special case of $n = 1$, while DFS corresponds to $n = \infty$. We tested versions of B-DFS$(n)$, $n = 1, 2, 3, 4, 5, 6, \infty$, and for all algorithms, ties during execution were broken randomly.

In addition to formulating the problem as search over a construal graph from the empty construal, we changed the goal from optimization (find the construal with the highest value) to satisficing (find a construal with value above a threshold). Specifically, once an algorithm finds any construal with a value above the threshold, it terminates and returns that construal. We used a satisficing approach for several reasons. First, without having a sense of what a "good" solution looks like in the form of a threshold or heuristic, search procedures like BFS, DFS, and B-DFS$(n)$ collapse into exhaustive enumeration. Second, we tested our approach on the mazes used in the experiments, in which solutions (construals and their associated plans) tended to cluster into those that reached the goal in a roughly optimal number of steps and those that did not reach the goal. Based on the size of the mazes, we chose a single value threshold of $-35$.

For each maze, we ran 500 simulations of the exhaustive enumeration procedure and the B-DFS$(n)$ procedures. For measures of the cost of the construal optimization procedure, we

recorded the number of construals that were evaluated (i.e., the total number of unique calls to a planning routine) and the size of the largest construal evaluated. To assess the quality of the solutions, we recorded the behavioral utility of the returned construals ($U(\pi_c)$) and their size ($C(c) = |c|$). Results for these four quantities, averaged over all algorithms and mazes, are plotted in Supplementary Figure 4. Results for individual mazes are shown in Supplementary Figure 5.

## 2.3 Results and discussion

We begin by discussing the behavior of BFS—i.e., B-DFS$(1)$. Qualitatively, BFS is a conservative approach to searching for satisficing construals. In particular, because BFS evaluates all construals of a certain size before testing larger construals, it is guaranteed to never evaluate a construal larger than the smallest satisficing construal, but tends to evaluate more construals. Even so, on 8 of the 16 mazes used in our experiments, BFS finds a satisficing construal in fewer than half of the number of average evaluations as the exhaustive algorithm. Thus, even when using a conservative search process that does not rely on a domain-specific heuristic, it is possible to noticeably improve over exhaustive search.

Would a more sophisticated construal search procedure perform better? As $n$ increases, the search process induced by B-DFS$(n)$ becomes more aggressive, meaning that it increases the size of evaluated construals more quickly (e.g., in the limit, DFS often evaluates and returns the full construal since it always adds a new effect to the construal). As can be seen in Supplementary Figure 5, increasing $n$ leads to a smaller *number of construals evaluated* but a larger *maximum evaluated construal size* and larger *returned construal size*. We considered what would happen if the decision-maker could select a bounded depth $n$ based on an estimate of the size of the optimal construal $|c^*|$ (this estimate could be guided by perceptual cues, like the amount of clutter in a maze). When $n = |c^*|$, we found that across the 16 mazes, the average number of evaluated construals ranged from $5\%$ to $49\%$ of the construals evaluated by the exhaustive algorithm.

Beyond the specific construal search procedures we explore here, there exist a large number

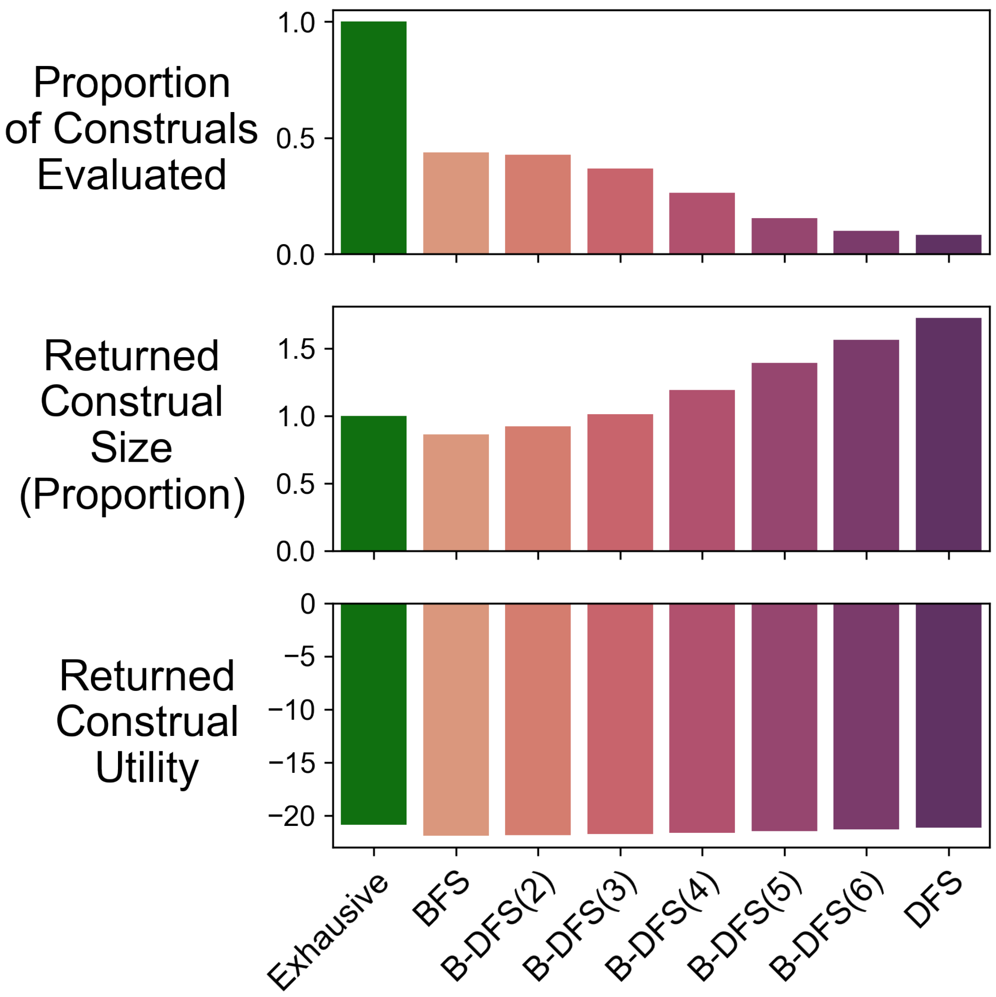


**Supplementary Figure 4:** Construal search simulations averaged over all 16 mazes ($N = 500$ independent simulations per maze). Although our primary focus is on whether people optimally form construals, an important theoretical question is the computational tractability of construal optimization. Here, we compare the number of construals evaluated under the theoretically optimal model (exhausive search over all construals) to several variants of breadth-first search (BFS) and depth-first search (DFS) that start from an empty construal and terminate when a satisficing construal is found. Top: Following a pure BFS construal evaluation order results in less than half as many construals being evaluated than exhaustive enumeration. When more DFS-like search is used, an even smaller proportion will be evaluated. Middle: BFS returns a satisficing construal that is at least as small as exhaustive search (smaller, but lower value construals could be returned if the value is less than optimal but above the threshold). As search becomes more depth-first, construals are less optimal, illustrating one way in which construal optimality and computation could trade off. Bottom: All models returned construals with roughly equivalent utility. *Exhaustive* = exhaustive search over all construals (i.e., subsets of effects); *BFS* = breadth-first search; *B-DFS*$(i)$ = bounded depth-first search up to a depth $i$; *DFS* = depth-first search.

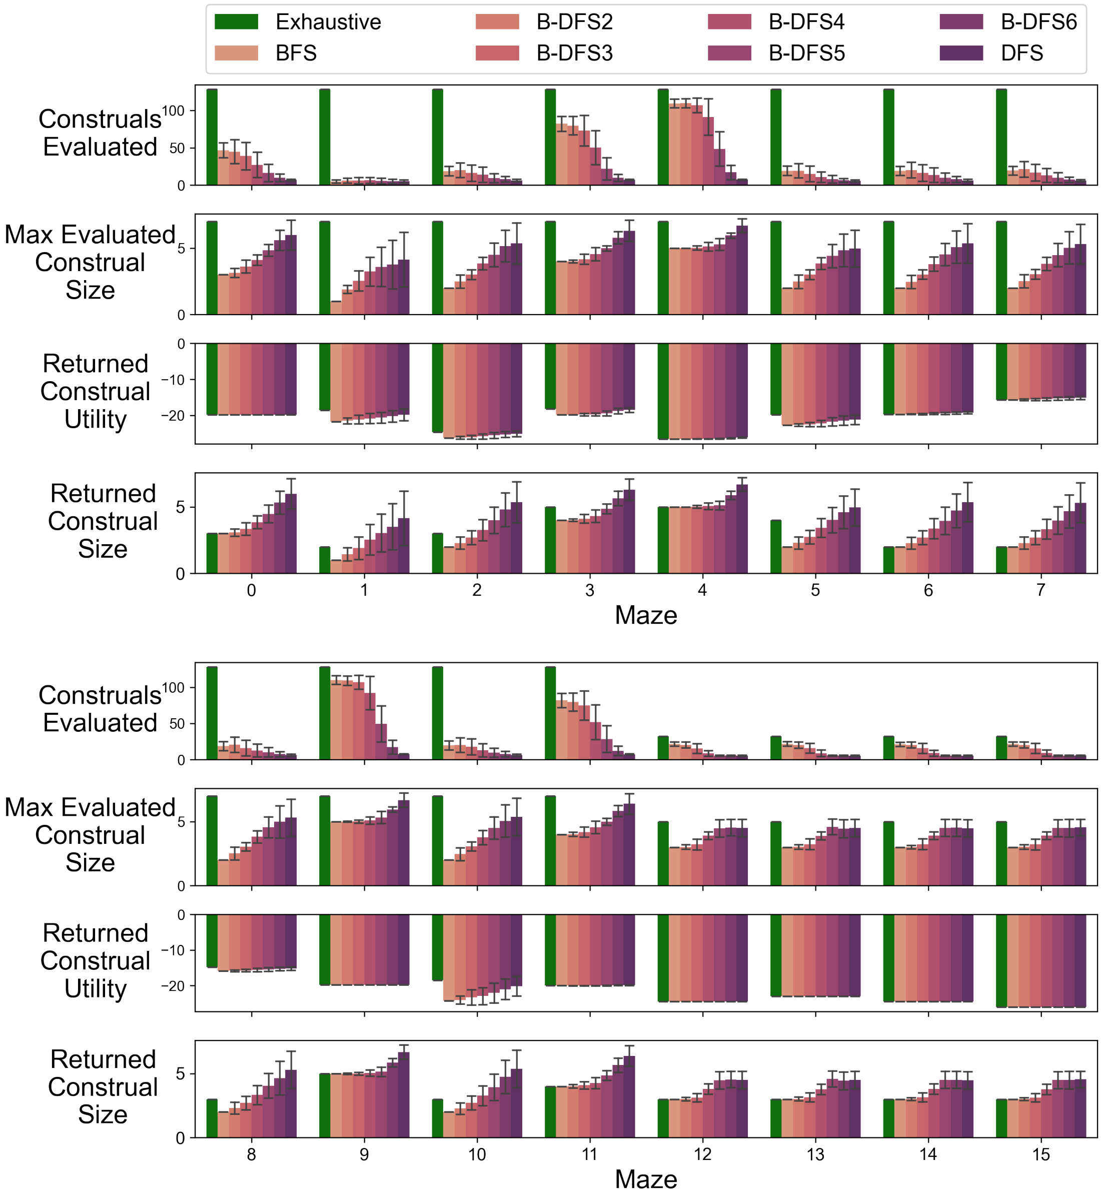


**Supplementary Figure 5:** Average quantities for construal search simulations for mazes 0-7 (top 3 rows) and mazes 8-15 (bottom 3 rows). Comparing the number of construals evaluated (first and fourth rows) with the path length of the resulting plan (second and fifth rows) and the size of the satisficing construal (third and sixth rows) demonstrates that in many cases, even uninformed search is a tractable method for optimizing construals that balance behavioral utility and the size of a construal. *Exhaustive* = exhaustive search over all construals (i.e., subsets of effects); *BFS* = breadth-first search; *B-DFS*$(i)$ = bounded depth-first search up to a depth $i$; *DFS* = depth-first search. Each bar represents the average of $N = 500$ independent simulations and error bars are standard deviations around the mean.

of alternative procedures. For instance, people could leverage domain-specific heuristics to guide the evaluation order or use perceptual cues to filter out unpromising construals. Our primary goal in this section has been to provide a minimal demonstration of how our framework can be extended to analyze the tractability of different construal optimization algorithms. Future research can build on the approach taken here to study the mechanisms that enable people construct task representations in an approximately optimal but procedurally tractable manner.

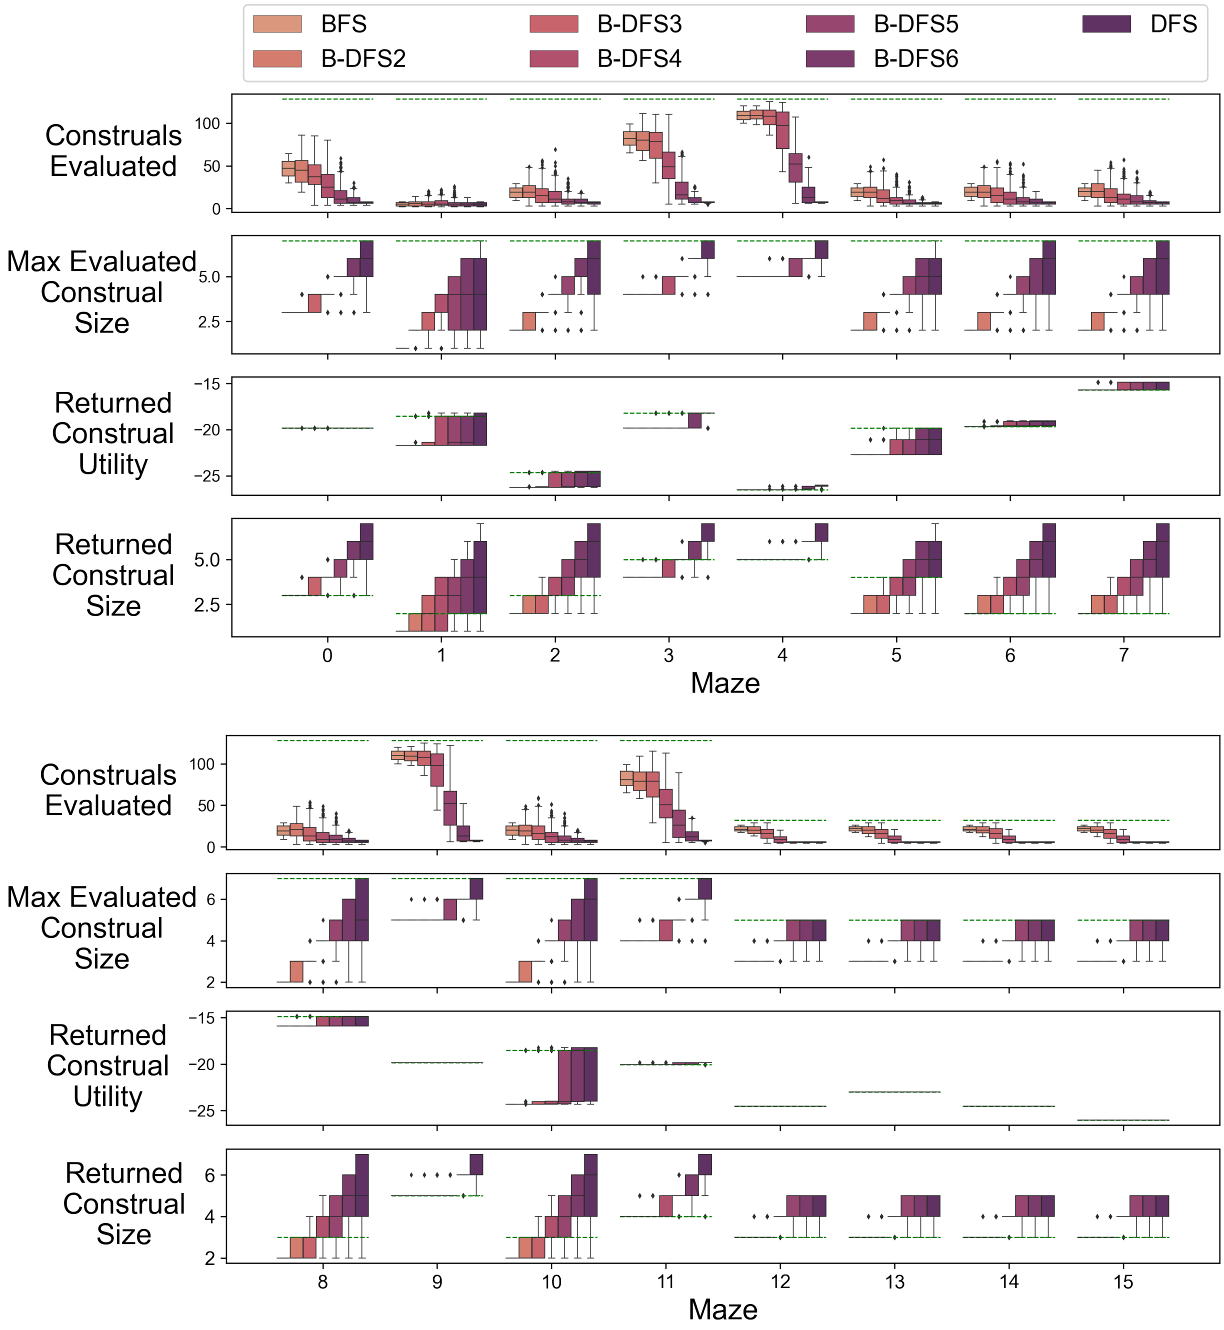


**Supplementary Figure 6:** Box and whisker plots for construal search simulations for mazes 0-7 (top 3 rows) and mazes 8-15 (bottom 3 rows). Boxes range from the 1st quartile to the 3rd quartile, whiskers are extended 1.5 times the inter-quartile range or until the furthest datapoint (whichever is closer). Outliers beyond 1.5 times the inter-quartile range are marked with small diamonds. Each boxplot corresponds to the results of $N = 500$ independent simulations. Dotted green lines correspond to the quantity using an exhaustive search algorithm.

# 3 Supplementary Experimental Materials

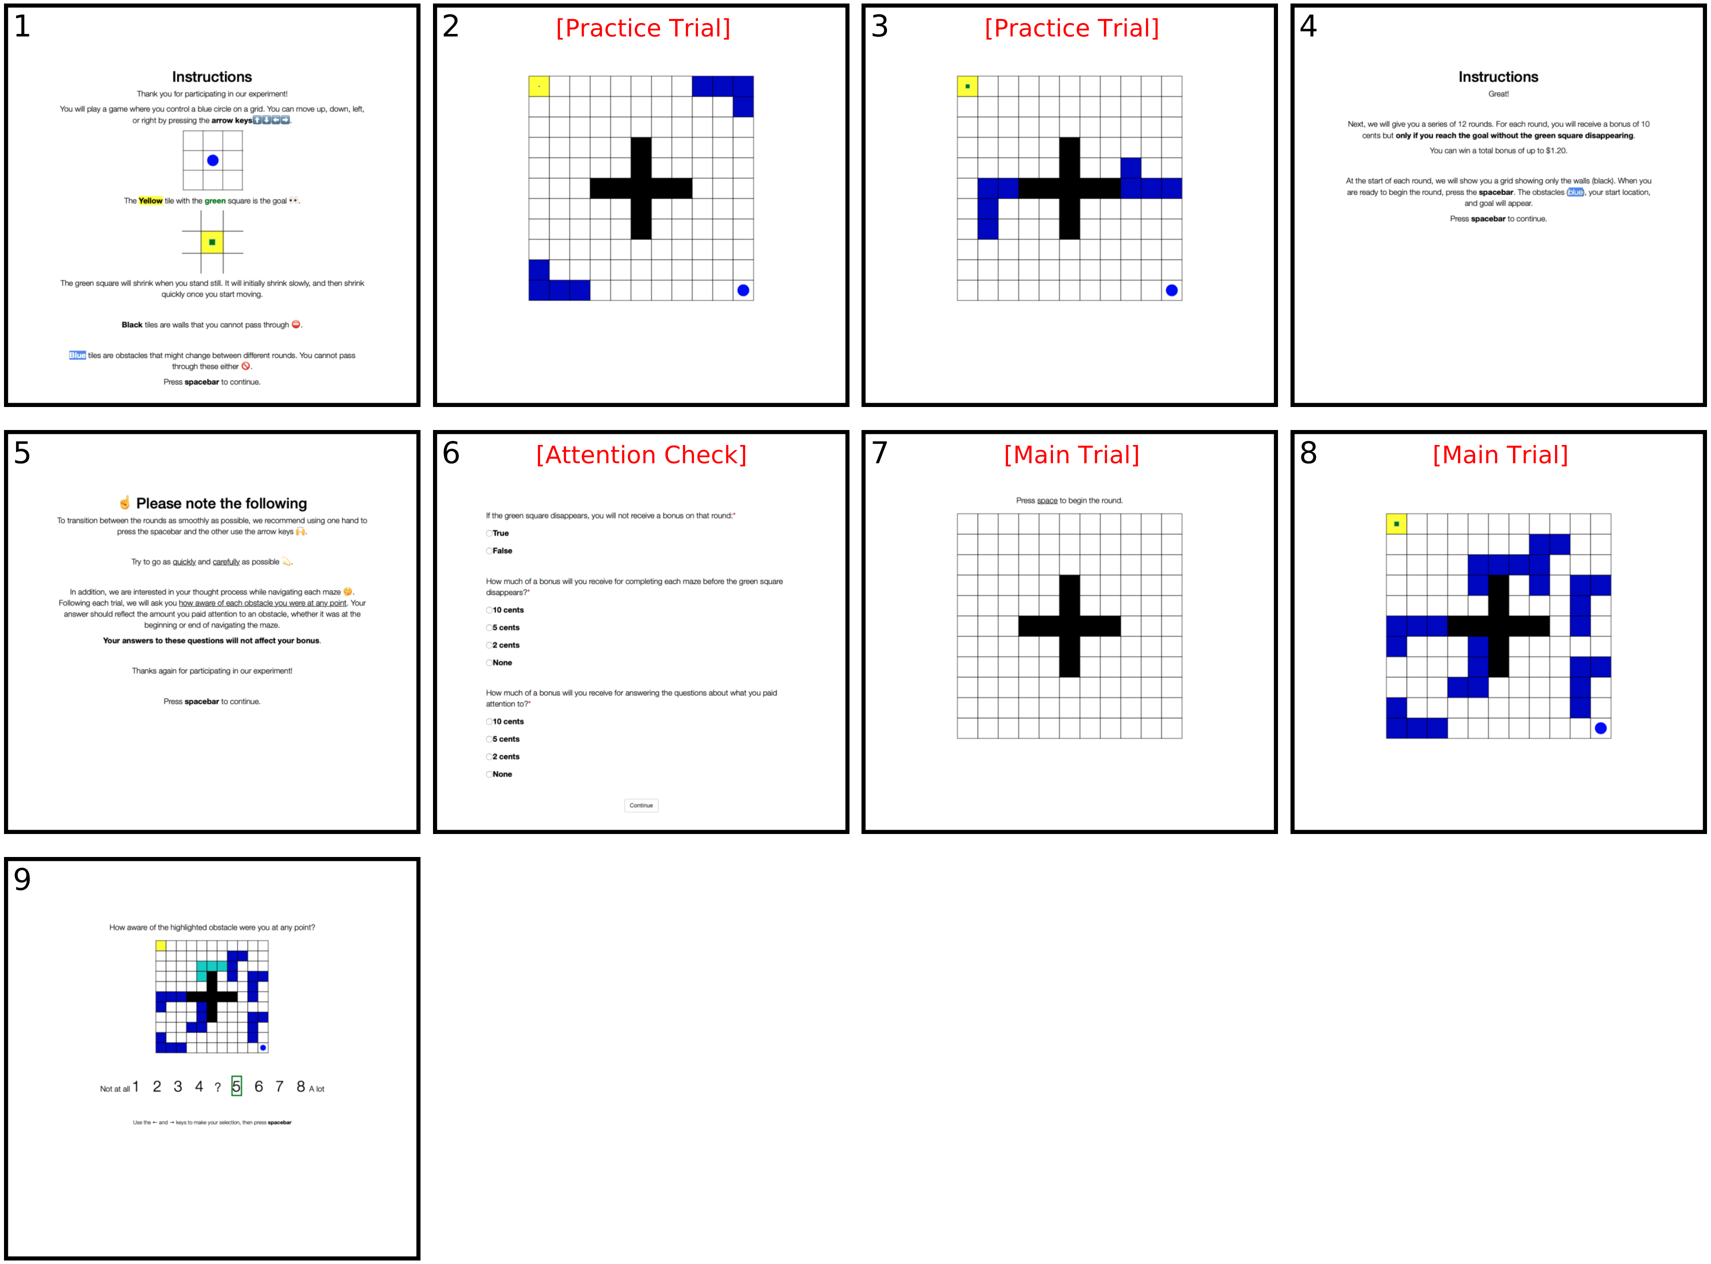


**Supplementary Figure 7:** Experiment 1 instructions and trial examples (red text not shown to participants).

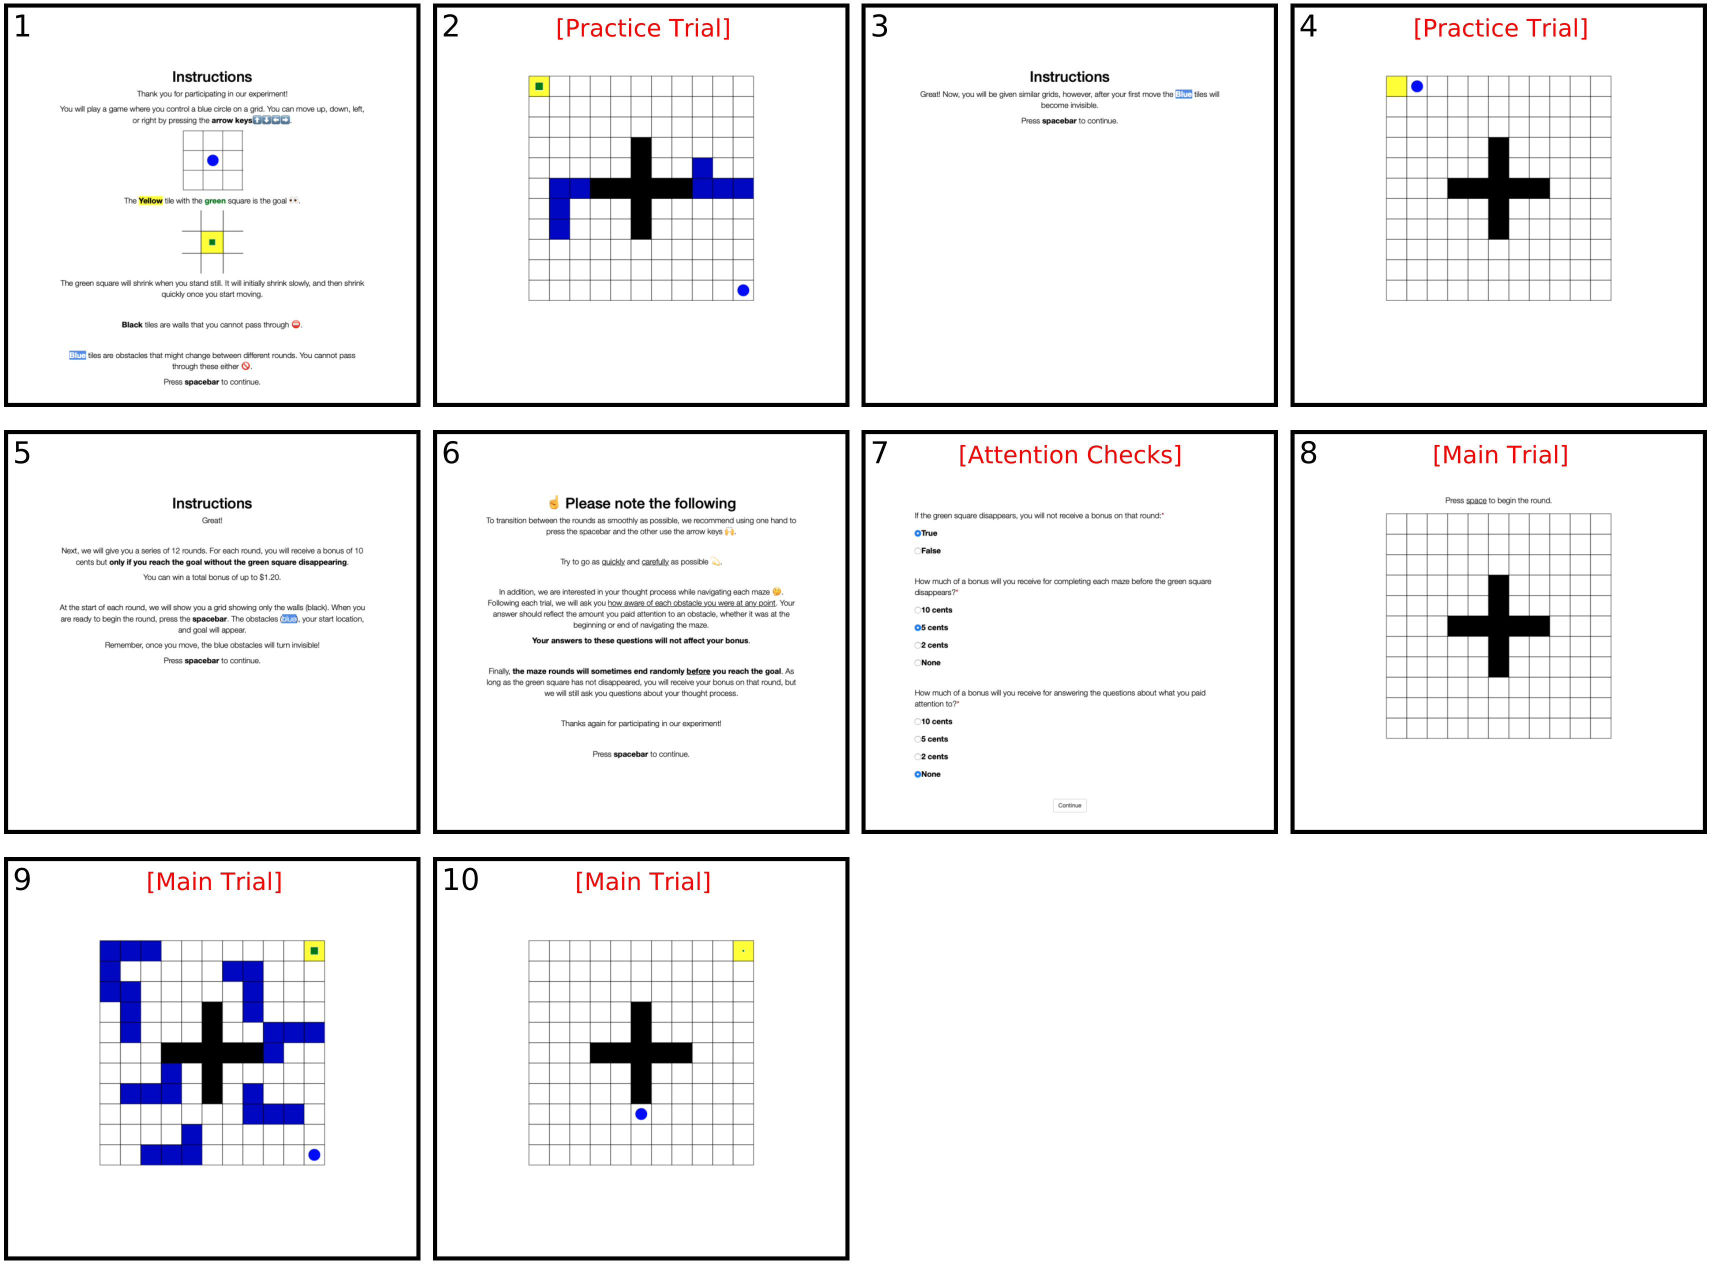


**Supplementary Figure 8:** Experiment 2 instructions and trial examples (red text not shown to participants).

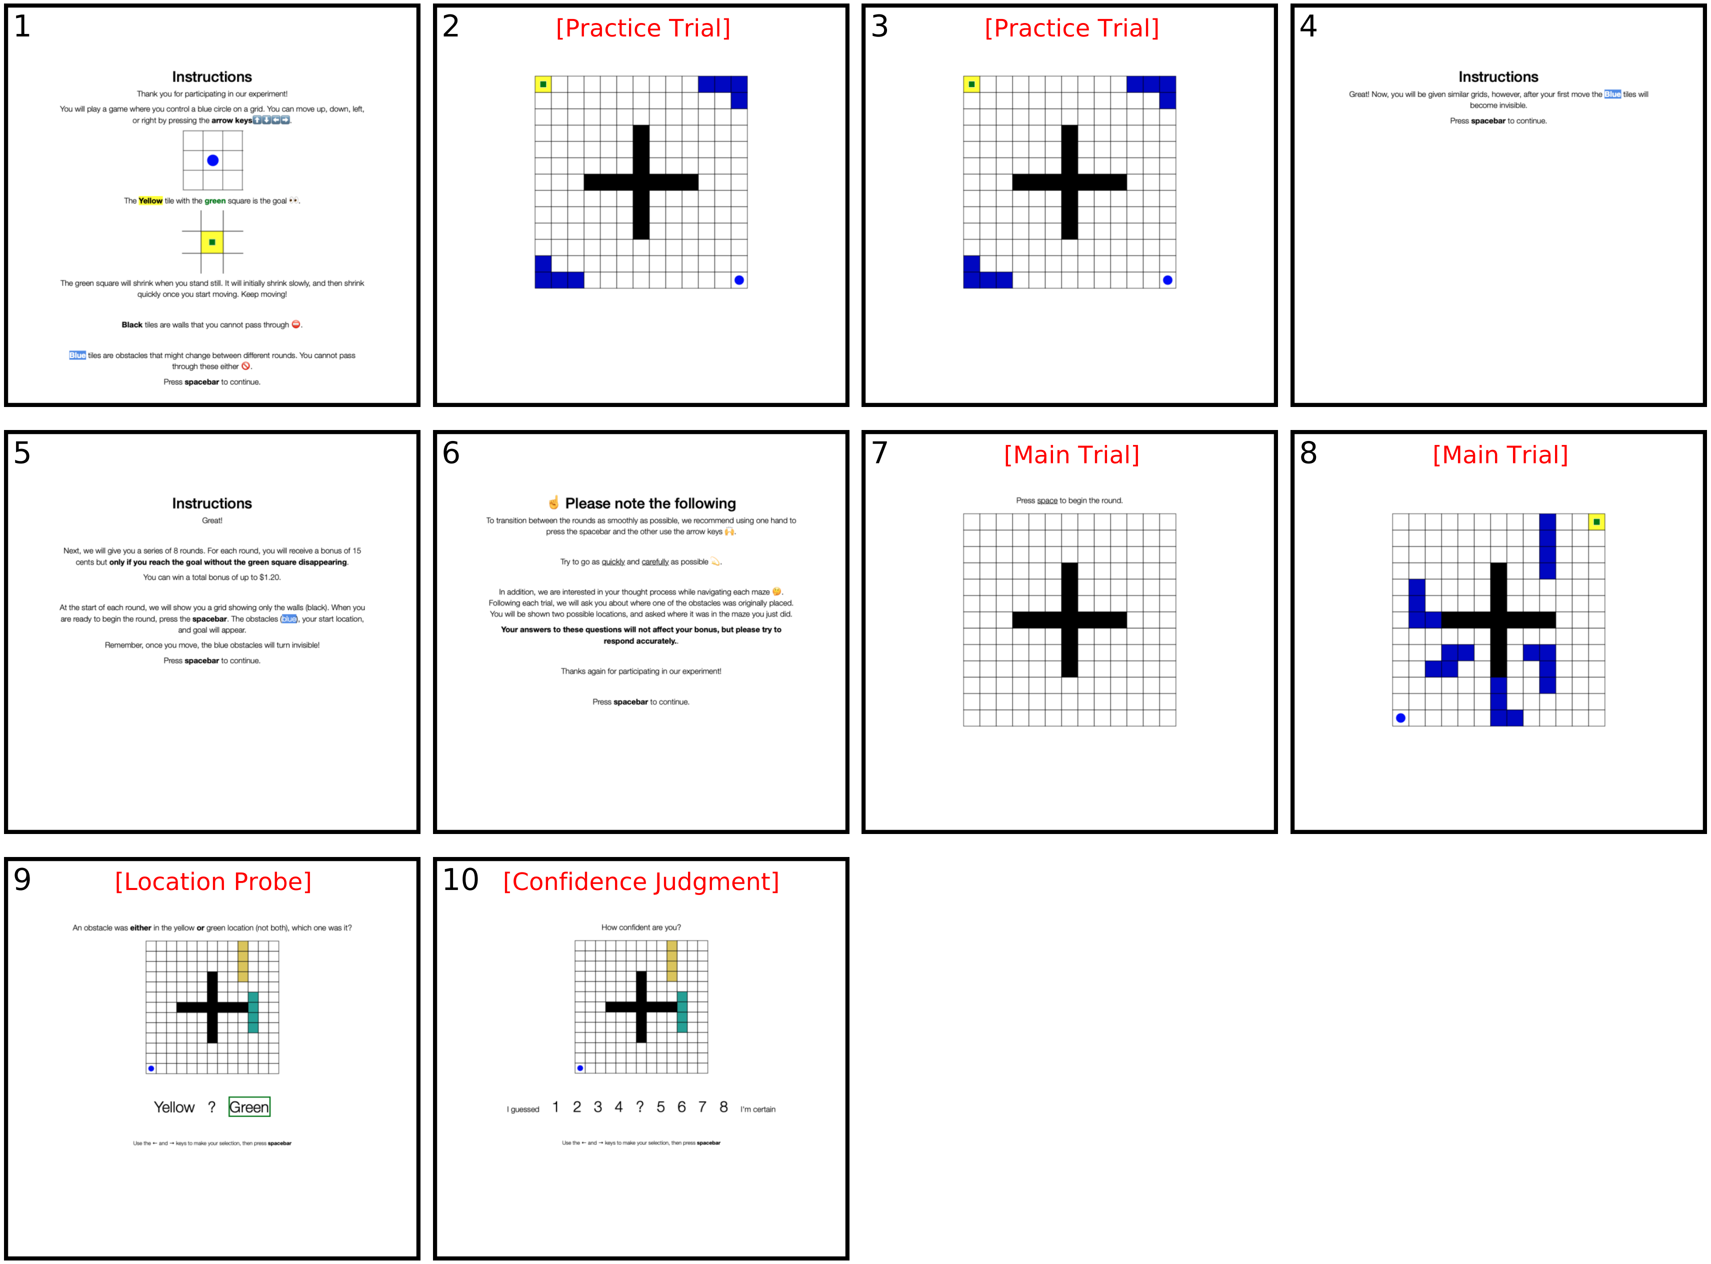


**Supplementary Figure 9:** Experiment 3 recall probe condition instructions and trial examples (red text not shown to participants).

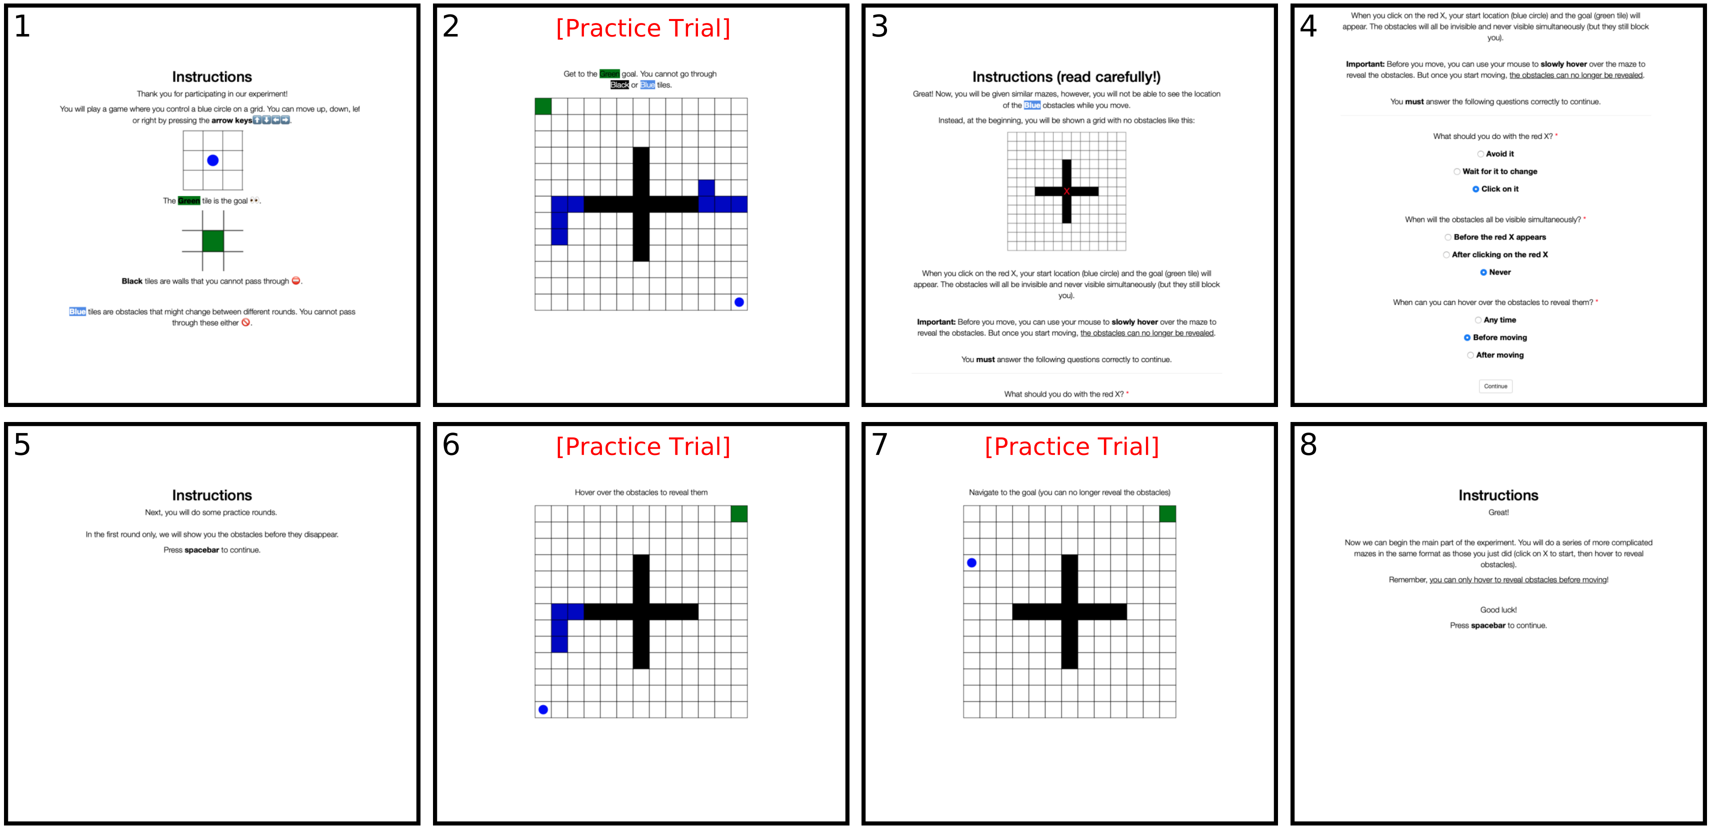


**Supplementary Figure 10:** Experiment 4 instructions and trial examples (red text not shown to participants).

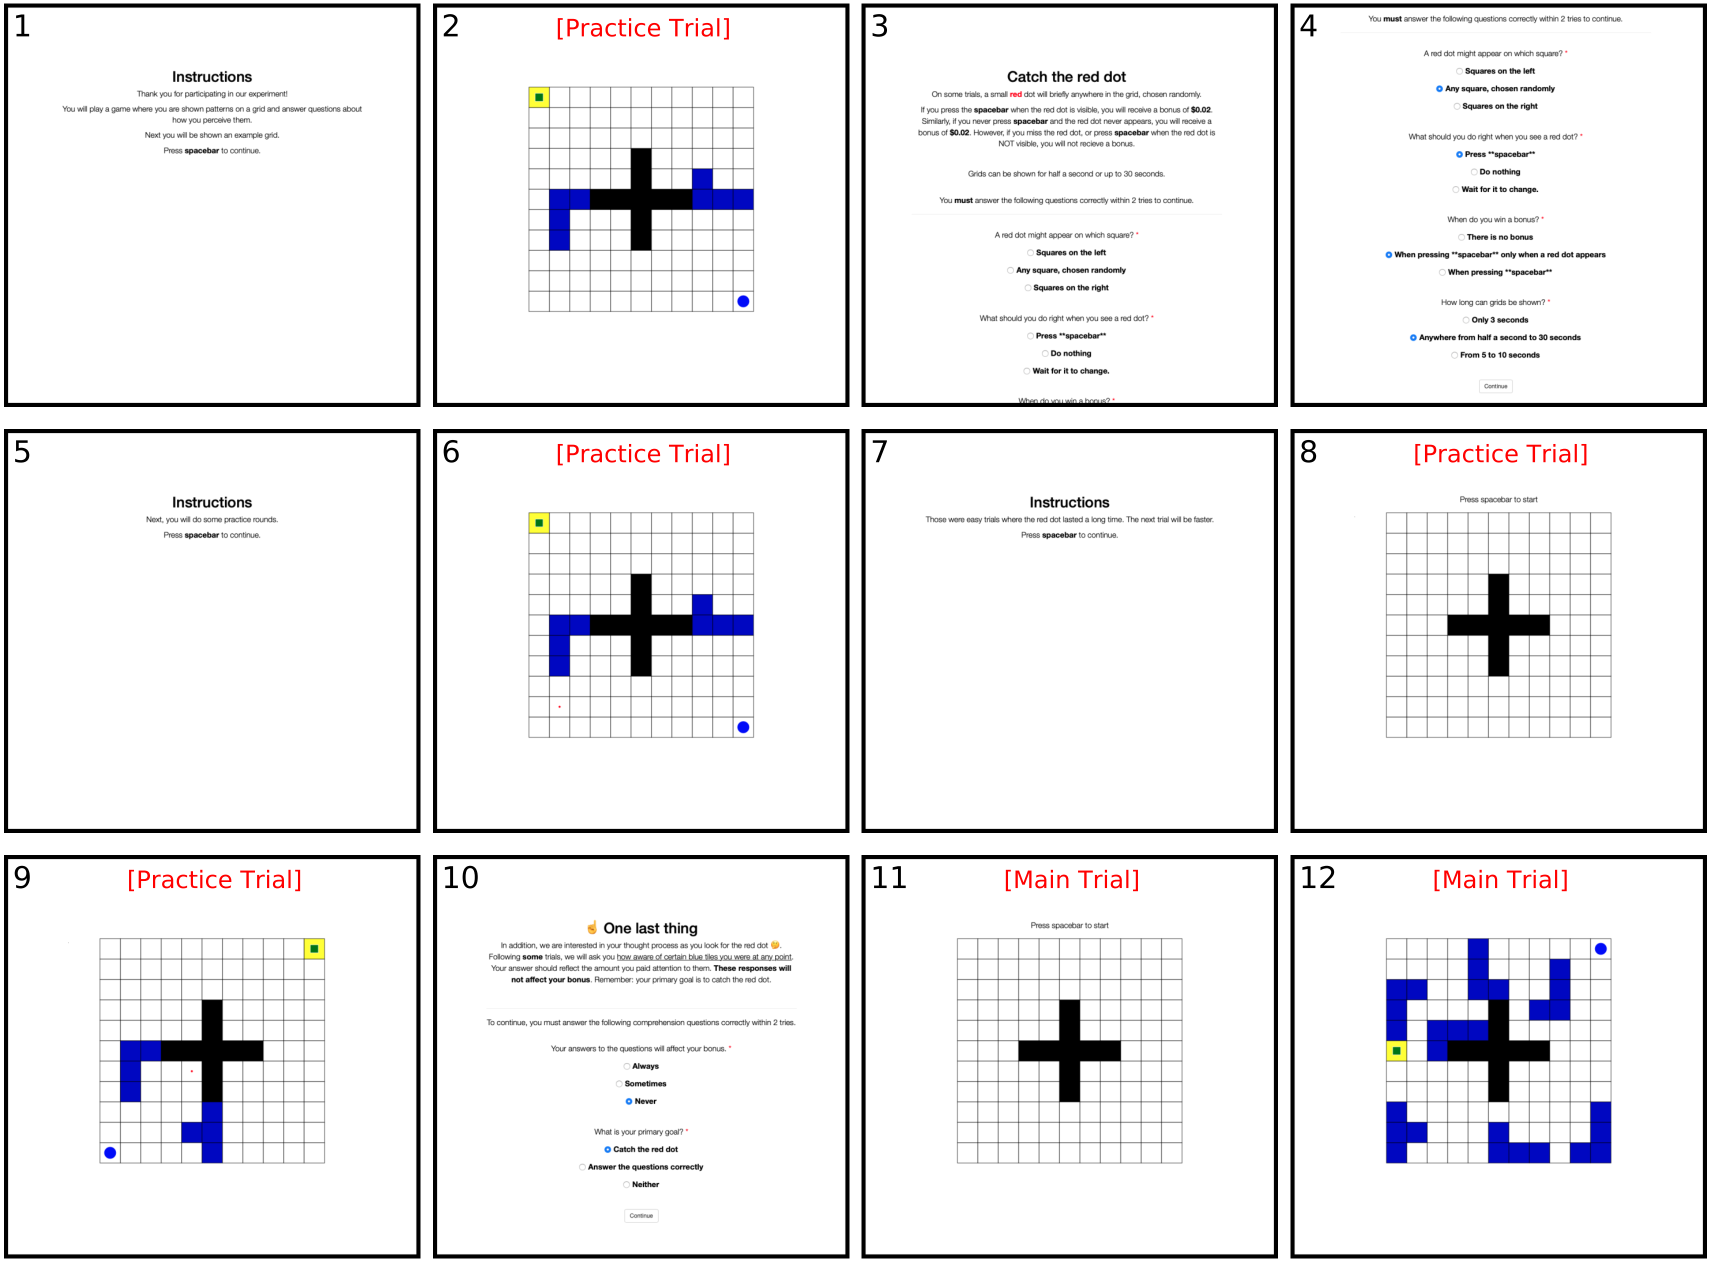


**Supplementary Figure 11:** Experiment 5 instructions and trial examples (red text not shown to participants).

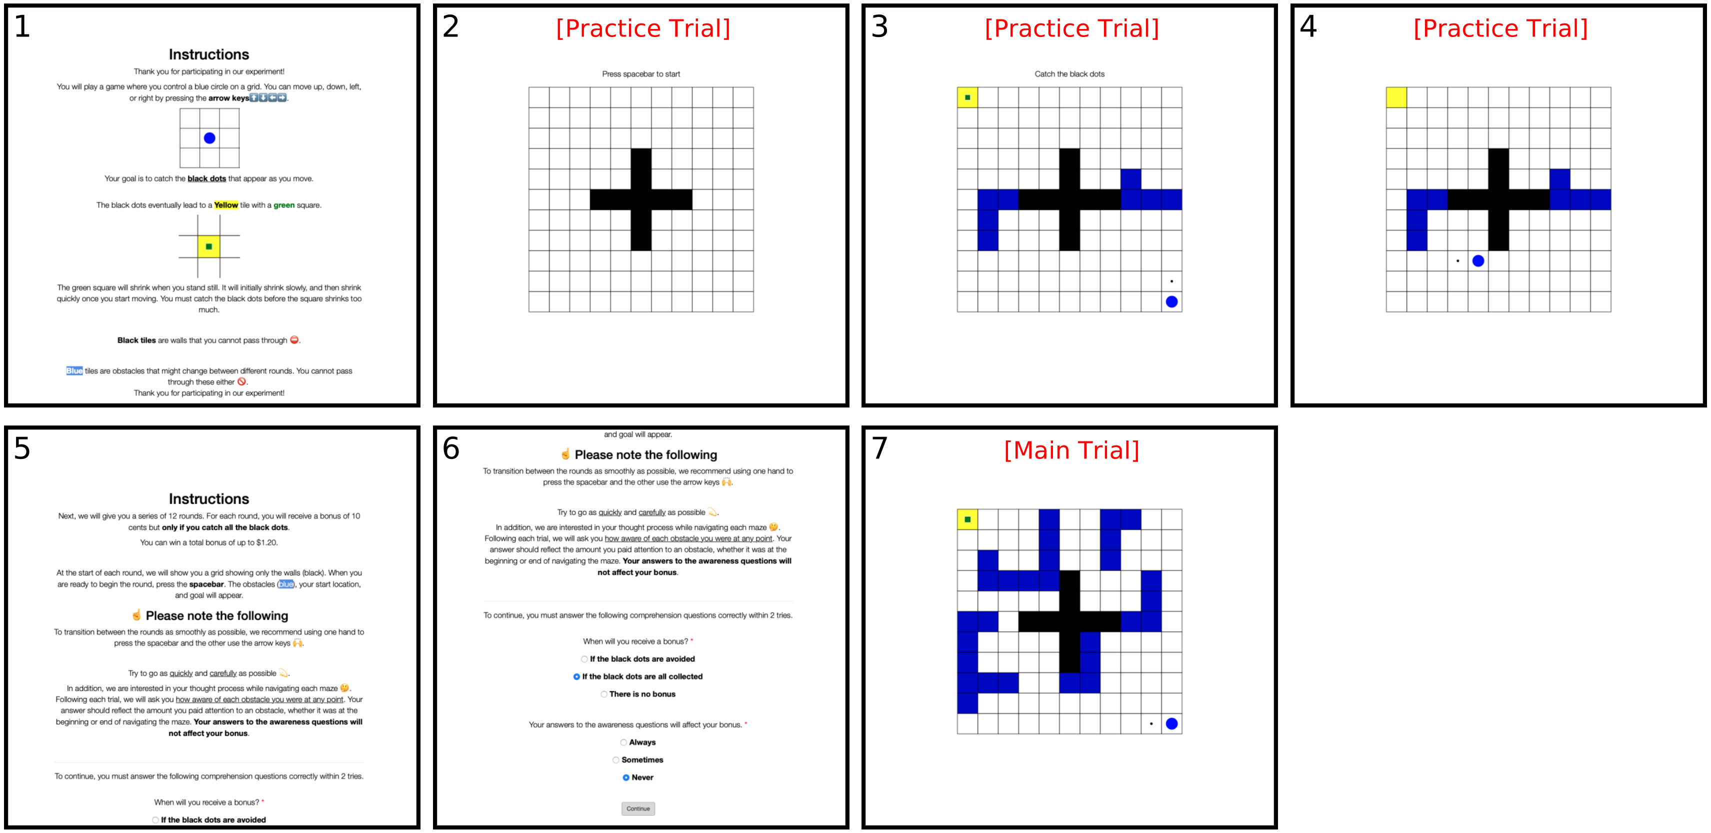


**Supplementary Figure 12:** Experiment 6 instructions and trial examples (red text not shown to participants).

# Supplementary Information References


1. Marr, D. *Vision: A computational investigation into the human representation and processing of visual information* (San Francisco: W. H. Freeman and Company, 1982).
2. Anderson, J. R. *The Adaptive Character of Thought* (Lawrence Erlbaum Associates, Inc., Hillsdale, NJ, 1990).
3. Griffiths, T. L., Lieder, F. & Goodman, N. D. Rational Use of Cognitive Resources: Levels of Analysis Between the Computational and the Algorithmic. *Topics in Cognitive Science* **7,** 217–229 (2015).
4. Simon, H. A. Rational choice and the structure of the environment. *Psychological review* **63,** 129 (1956).
